# Supplementary material for: Geometric Adversarial Attacks and Defenses on 3D Point Clouds
Source: arXiv:2012.05657 source file (2021-10-16)
Supplement: Supplementary file 1 [file classification_two_examples.tex]

\begin{figure}[tb!]
\begin{center}
\begin{tabular}{ c c c }
Clean  & Output space & Clean  \\
source & attack       & target \\

\includegraphics[width=0.28\linewidth]{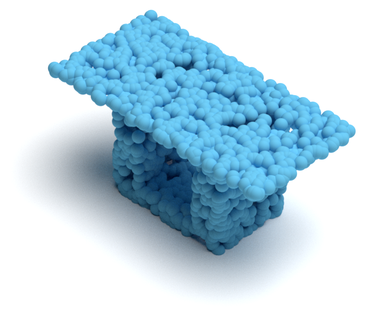} &
\includegraphics[width=0.28\linewidth]{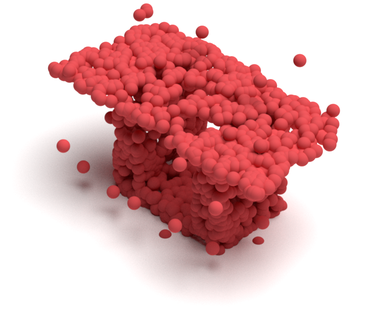} &
\includegraphics[width=0.28\linewidth]{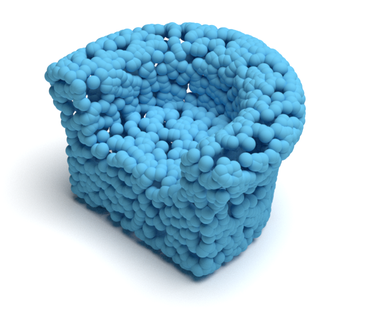} \\

\includegraphics[width=0.28\linewidth]{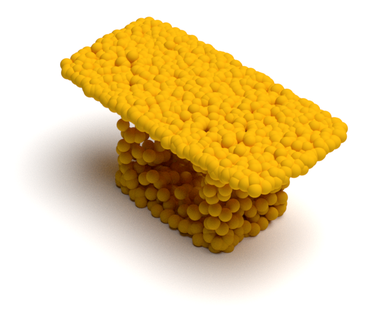} &
\includegraphics[width=0.28\linewidth]{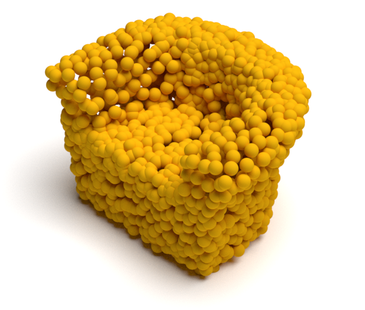} &
\includegraphics[width=0.28\linewidth]{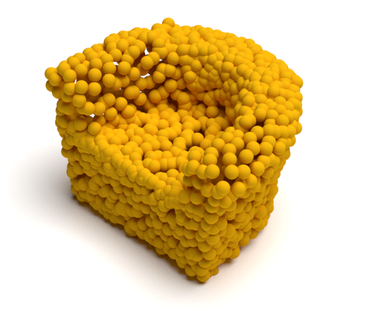} \\

Reconstructed & Reconstructed     & Reconstructed \\
source        & adversarial input & target        \\
Label: \textit{table} & Label: \textit{sofa} & Label: \textit{sofa} \\
Pred: \textit{table} & Pred: \textit{chair} & Pred: \textit{chair}

\\
\\

Clean  & Output space & Clean  \\
source & attack       & target \\

\includegraphics[width=0.28\linewidth]{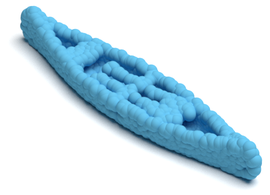} &
\includegraphics[width=0.28\linewidth]{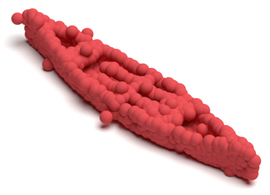} &
\includegraphics[width=0.28\linewidth]{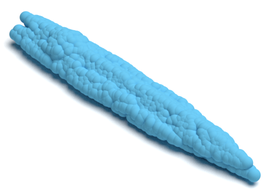} \\

\includegraphics[width=0.28\linewidth]{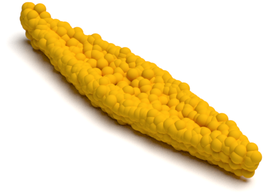} &
\includegraphics[width=0.28\linewidth]{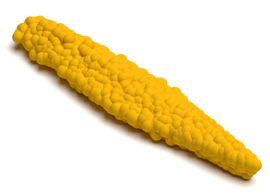} &
\includegraphics[width=0.28\linewidth]{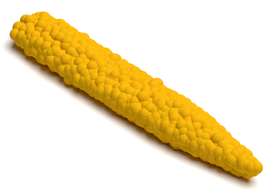} \\

Reconstructed & Reconstructed     & Reconstructed \\
source        & adversarial input & target        \\
Label: \textit{watercraft} & Label: \textit{airplane} & Label: \textit{airplane} \\
Pred: \textit{watercraft} & Pred: \textit{watercraft} & Pred: \textit{watercraft}

\end{tabular}
\caption{{\bfseries Target shapes with wrong semantic interpretation.} The first row in each group: a clean source point cloud, an adversarial example, and a clean target. The second row in each group: the corresponding reconstructions. Below the reconstructed point clouds, we indicate their shape class (Label) and predicted label (Pred) by a classifier. Our attack may select targets that are wrongly classified, though the classifier's mistake is reasonable.}
\label{fig:supp_classification}
\end{center}
\end{figure}
