# Supplementary material for: Geometric Adversarial Attacks and Defenses on 3D Point Clouds
Source: arXiv:2012.05657 source file (2021-10-16)
Supplement: Supplementary file 2 [file defense_latent.tex]

\begin{figure*}[tb!]
\begin{center}
\begin{tabular}{ c c c c  c }
Clean  & Latent space & Off-surface    & Critical points & Clean  \\
source & attack       & defense           & defense         & target \\

\includegraphics[width=0.17\linewidth]{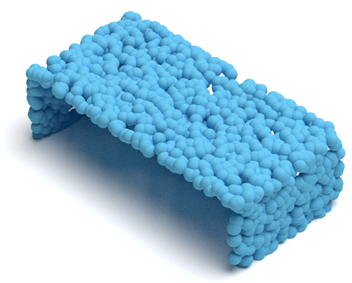} &
\includegraphics[width=0.17\linewidth]{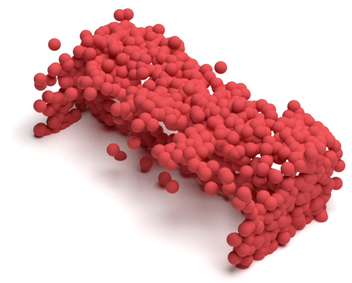} &
\includegraphics[width=0.17\linewidth]{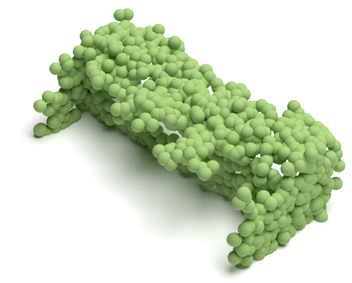} &
\includegraphics[width=0.17\linewidth]{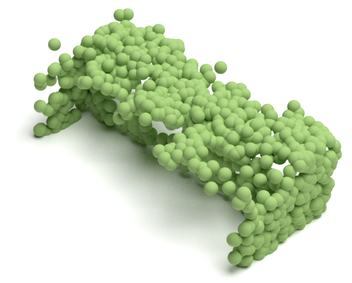} &
\includegraphics[width=0.17\linewidth]{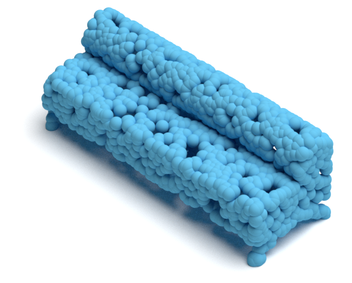} \\

\includegraphics[width=0.17\linewidth]{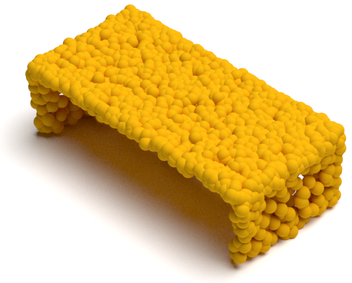} &
\includegraphics[width=0.17\linewidth]{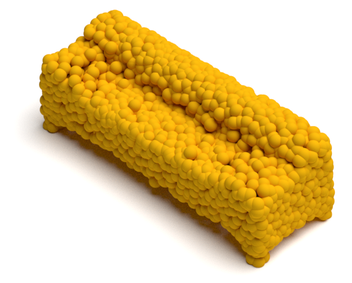} &
\includegraphics[width=0.17\linewidth]{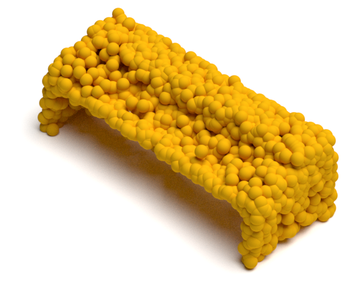} &
\includegraphics[width=0.17\linewidth]{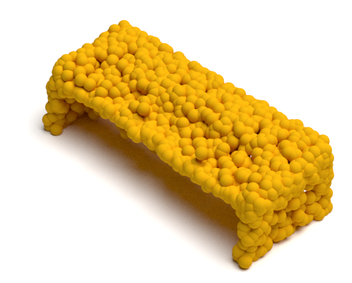} &
\includegraphics[width=0.17\linewidth]{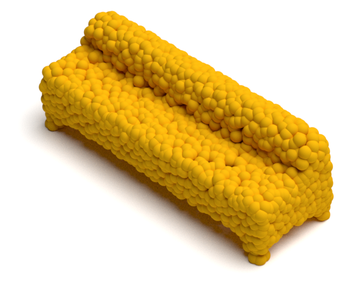} \\

Reconstructed  & Reconstructed     & Reconstructed  & Reconstructed  & Reconstructed \\
source         & adversarial input & defended input & defended input & target        \\
$\SNRE = 1.00$ & $\SNRE = 9.62$    & $\SNRE = 5.56$ & $\SNRE = 4.37$ & N/A           \\
\end{tabular}
\caption{{\bfseries Defense for the targeted latent space attack.} Top row: a clean source point cloud (\textit{table}), an adversarial example of the targeted latent space attack, defended point cloud by the off-surface defense, defended point cloud by the critical points defense, and a clean target (\textit{sofa}). Bottom row: corresponding reconstructions and their source normalized reconstruction error, $\SNRE$ (not applicable for the reconstructed target). After the defense, remnants of the attack are still much present at the reconstructed output.}
\label{fig:supp_defense_latent}
\end{center}
\end{figure*}
