# Supplementary material for: Geometric Adversarial Attacks and Defenses on 3D Point Clouds
Source: arXiv:2012.05657 source file (2021-10-16)
Supplement: Supplementary file 4 [file correct_targets.tex]

\begin{table}[tb!]
\begin{center}
\begin{tabular}{ l c c c c }
\hline
\multicolumn{5}{c}{Attack Results with Semantic Consideration} \\
Attack Type  & \#$OS$  & $\SCD$ & $\TRE$ & $\TNRE$  \\
%\\
\hline
\hline
%\\
Latent (Tgt) & 32 & 0.81 & 1.05 & 1.75 \\
Output (Tgt) & 25 & 0.49 & 0.63 & 1.14 \\
%Output (Tgt) & {\bfseries 25} & {\bfseries 0.49} & {\bfseries 0.63} & {\bfseries 1.14} \\
%\\
\hline
%\\
%Latent (unTgt) & 18 & 0.34 & 0.44 & 1.08 \\
%Output (unTgt) & {\bfseries 13} & {\bfseries 0.16} & {\bfseries 0.34} & {\bfseries 0.91} \\
%\\
%\hline
%\\
\end{tabular}
\end{center}
\caption{{\bfseries Geometric adversarial metrics for correctly classified targets.} The acronyms are the same as in Table~\ref{tbl:attacks_loss_dist_chamfer} in the paper. The $\SCD$ and $\TRE$ are multiplied by a factor of $10^3$. Lower is better. Selecting targets for the attacks with correct semantic interpretation decrease the attacks' geometric performance.}
\label{tbl:supp_attacks_correct_targets}
\end{table}
